# Supplementary material for: An Equivalent Circuit Approach to Distributed Optimization
Source: arXiv:2305.14607 source file (2023-05-24)
Supplement: Supplementary file 6 [file distributed_ec_model_old.tex]

\section{Distributed Equivalent Circuit Model}

In this section, we design an equivalent circuit model of the optimization problem in (XX). First, we define a continuous-time version of gradient descent, known as scaled gradient-flow, from which we derive the equivalent circuit model. Scaled gradient-descent a continuous-time ODE that models the trajectory of the optimization variable, $x$ to a critical point. The scaled gradient flow is defined as:
\begin{equation}
    Z(x(t))\dot{x}(t) = -\nabla f(x(t))
    \label{eq:gd_flow}
\end{equation}
where $Z(x(t))$ is a diagonal matrix that scales the components of the gradient to modify the overall trajectory. Further derivation and proof of convergence is defined in (XX).

For the separable optimization problem in (XX), the scaled-gradient flow is defined as:
\begin{equation}
    Z(x(t))\dot{x}(t) = -\sum_{i=1}^{n} \nabla f_i (x(t))
    \label{eq:seperable_gd_flow}
\end{equation}

The equivalent circuit model of \ref{eq:gd_flow} is namely defined by two circuit components: a nonlinear capacitor with capacitance $Z(x)$ and a voltage-controlled current source (VCCS). The VCCS element produces a current equal to to $\nabla f(x)$.



The equivalent circuit model of the separable problem in \ref{eq:seperable_gd_flow} has a similar structure, but the VCCS element that produces $\nabla f(x)$ is now separated into $n$ parallel VCCS components, each delivering current of $\nabla f_i (x(t))$. As shown in Figure XX, the EC model of \ref{eq:seperable_gd_flow} shares a common node voltage, $x$.


\subsection{Distributing the Node Voltage}

The goal of distributed optimization is to partition the optimization objective, $f(x)$ into $n$ sub-problems. Each sub-problem, $f_i(x)$, is solved locally and communicates the local updates to $x$ to the centralized controller. To achieve this in the EC framework, we perform two modifications to the underlying EC model:\\
1) add an added capacitor, $Z_c$, whose voltage represents the state variable $x$ for the centralized controller \\
2) add small resistances between the centralized node and each sub-problem.

To begin, first split the capacitor, $Z(x)$ into $n+1$ parallel capacitors for each sub-problem and the central node. The capacitor at the central node has a capacitance denoted, $Z_c(x)$, and the capacitor at each sub-problem has a capacitance of $Z_i(x)$. Overall,  is defined as:
\begin{equation}
    Z(x) = \sum_{i=1}^{n} Z_i(x)
\end{equation}
